# Supplementary material for: An Empirical Study of Blockchain System Vulnerabilities: Modules, Types, and Patterns
Source: arXiv:2110.12162 source file (2023-02-21)
Supplement: Supplementary file 1 [file appendix.tex]

\section*{Appendix}
\appendix
\section{Supplementary Patch Examples}
\label{sec:appendix1}

In this section, we provide eight supplementary patch code examples for the contents in \mysec\ref{subsec:code_pattern}.
Specifically, Table~\ref{tab:p2exp}, \ref{tab:p4exp}, \ref{tab:p7exp}, \ref{tab:p8exp}, \ref{tab:p11exp}, \ref{tab:p19exp}, \ref{tab:p20exp}, and \ref{tab:p21exp} describe the patch code examples for the pattern P2, P4, P7, P8, P11, P19, P20, and P21, respectively.

%\vspace{-1.5em}
\begin{table}[h!]
	\centering
	\caption{A patch code example of P2, Bitcoin \#2273}
	\label{tab:p2exp}
    \vspace{-2ex}
	% \resizebox{\linewidth}{!}{%
	\begin{adjustbox}{center} %angle=90
	\scalebox{0.7}{
		\begin{tabular}{c|l|}
			% \multicolumn{2}{l}{Bitcoin commit 5d322821:} \\
			\cline{2-2}
			  & \texttt{bool CTransaction::IsStandard() const \{}                                   \\
			  & \texttt{\hspace{5mm}...}                                                        \\
			+ & \texttt{\hspace{5mm}// Extremely large txns with lots of inputs can cost the network} \\
			+ & \texttt{\hspace{5mm}// almost as much to process as they cost the sender in fees, because} \\
			+ & \texttt{\hspace{5mm}// computing signature hashes is O(ninputs*txsize). Limiting txns} \\
			+ & \texttt{\hspace{5mm}// to MAX\_STANDARD\_TX\_SIZE mitigates CPU exhaustion attacks.} \\
			+ & \texttt{\hspace{5mm}unsigned int sz = this->GetSerializeSize(...);}          \\
			+ & \texttt{\hspace{5mm}if (sz >= MAX\_STANDARD\_TX\_SIZE)}                 \\
			+ & \texttt{\hspace{10mm}return false;}                 \\
			  & \texttt{\hspace{5mm}...}  \\
			  & \texttt{\}} \\
		    \cline{2-2}                                                                   
		\end{tabular}%
	}
	\end{adjustbox}
\end{table}

\begin{table}[h!]
	\centering
	\caption{A patch code example of P4, Bitcoin \#1167}
	\label{tab:p4exp}
    \vspace{-2ex}
	% \resizebox{\linewidth}{!}{%
	\begin{adjustbox}{center} %angle=90
	\scalebox{0.7}{
		\begin{tabular}{c|l|}
			% \multicolumn{2}{l}{Bitcoin commit 5d322821:} \\
			\cline{2-2}
			  & \texttt{bool CBlock::CheckBlock() const \{}       \\
			  & \texttt{\hspace{5mm}...}                                                        \\
			+ & \texttt{\hspace{5mm}// Check for duplicate txids. This is caught by ConnectInputs(),} \\
			+ & \texttt{\hspace{5mm}// but catching it earlier avoids a potential DoS attack:}          \\
			+ & \texttt{\hspace{5mm}set<uint256> uniqueTx;}                 \\
			+ & \texttt{\hspace{5mm}BOOST\_FOREACH(const CTransaction\& tx, vtx)}                                                                       \\
			+ & \texttt{\hspace{5mm}\{}                                                                       \\
		    + & \texttt{\hspace{10mm}uniqueTx.insert(tx.GetHash());}                                                                       \\
		    + & \texttt{\hspace{5mm}\}}                                                                       \\
		    + & \texttt{\hspace{5mm}if (uniqueTx.size() != vtx.size())}                                                                       \\
		    + & \texttt{\hspace{10mm}return DoS(100, error("CheckBlock() : duplicate transaction"));\hspace{4mm}}                                                                       \\
			  & \texttt{\hspace{5mm}...}  \\
			  & \texttt{\}} \\
		    \cline{2-2}                                                                   
		\end{tabular}%
	}
	\end{adjustbox}
\end{table}

\begin{table}[h!]
	\centering
	\caption{A patch code example of P7, Bitcoin \#11531}
	\label{tab:p7exp}
    \vspace{-2ex}
	% \resizebox{\linewidth}{!}{%
	\begin{adjustbox}{center} %angle=90
	\scalebox{0.7}{
		\begin{tabular}{c|l|}
			% \multicolumn{2}{l}{Bitcoin commit 5d322821:} \\
			\cline{2-2}
			  & \texttt{static bool AcceptBlockHeader(const CBlockHeader\& block, ...) \{}       \\
			  & \texttt{\hspace{5mm}...}                                                        \\
			  & \texttt{\hspace{5mm}if (!ContextualCheckBlockHeader(block, state, chainparams, ...))}                                                        \\
			  & \texttt{\hspace{10mm}return error("\%s: Consensus::ContextualCheckBlockHeader:", ...);}                                                        \\
			  & \texttt{\hspace{5mm}}                                                        \\
			+ & \texttt{\hspace{5mm}if (!pindexPrev->IsValid(BLOCK\_VALID\_SCRIPTS)) \{} \\
			+ & \texttt{\hspace{10mm}for (const CBlockIndex* failedit : g\_failed\_blocks) \{}          \\
			+ & \texttt{\hspace{15mm}if (pindexPrev->GetAncestor(failedit->nHeight) == failedit) \{}                 \\
			+ & \texttt{\hspace{20mm}assert(failedit->nStatus \& BLOCK\_FAILED\_VALID);}                                                                       \\
			+ & \texttt{\hspace{20mm}CBlockIndex* invalid\_walk = pindexPrev;}                                                                       \\
		    + & \texttt{\hspace{20mm}while (invalid\_walk != failedit) \{}                                                                       \\
		    + & \texttt{\hspace{25mm}invalid\_walk->nStatus |= BLOCK\_FAILED\_CHILD;}                                                                       \\
		    + & \texttt{\hspace{25mm}setDirtyBlockIndex.insert(invalid\_walk);}                                                                       \\
		    + & \texttt{\hspace{25mm}invalid\_walk = invalid\_walk->pprev;}                                                                       \\
		    + & \texttt{\hspace{20mm}\}}                                                                       \\
		    + & \texttt{\hspace{20mm}return state.DoS(100, error("\%s: prev block invalid", ...);}                                                                       \\
			  & \texttt{\hspace{5mm}...}  \\
			  & \texttt{\}} \\
		    \cline{2-2}                                                                   
		\end{tabular}%
	}
	\end{adjustbox}
\end{table}

\begin{table}[H]
	\centering
	\caption{A patch code example of P8, Ethereum \#389}
	\label{tab:p8exp}
    \vspace{-2ex}
	% \resizebox{\linewidth}{!}{
	\begin{adjustbox}{center} %angle=90
	\scalebox{0.7}{
		\begin{tabular}{c|l|}
			% \multicolumn{2}{l}{Ethereum commit b155b9d8:} \\
			\cline{2-2}
			  & \texttt{func (sm *BlockProcessor) ValidateBlock(block, parent *types.Block) error \{}                                                     \\
			  & \texttt{\hspace{5mm}...}         \\
			  %& \texttt{\hspace{5mm}if len(block.Header().Extra) > 1024 \{}         \\
			  %& \texttt{\hspace{10mm}return fmt.Errorf("Block extra data too long (\%d)", len(}                                                            \\
			  %& \texttt{\hspace{10mm}block.Header().Extra))}                        \\
			  %& \texttt{\hspace{5mm}\}}                                             \\
			  %& \texttt{\hspace{5mm}expd := CalcDifficulty(block, parent)}          \\
			  %& \texttt{\hspace{5mm}if expd.Cmp(block.Header().Difficulty) != 0 \{} \\
			  %& \texttt{\hspace{10mm}return fmt.Errorf("Difficulty check failed for block", ...)}                      \\
			  %& \texttt{\hspace{5mm}\}}                                                         \\
			  %&                                                                     \\
			+ & \texttt{\hspace{5mm}expl := CalcGasLimit(parent, block)}            \\
			+ & \texttt{\hspace{5mm}if expl.Cmp(block.Header().GasLimit) != 0 \{}   \\
			+ & \texttt{\hspace{10mm}return fmt.Errorf("GasLimit check failed for block", ...)}                          \\
			+ & \texttt{\hspace{5mm}\}}                                             \\
			+ &                                                                     \\
			  & \texttt{\hspace{5mm}if block.Time() < parent.Time() \{}             \\
			  & \texttt{\hspace{10mm}return ValidationError("Block timestamp not after prev block", ...)} \\
			  & \texttt{\hspace{5mm}\}}                                             \\
			  & \texttt{\hspace{5mm}...}                                            \\
			  & \texttt{\}} \\
			\cline{2-2}                                                       
		\end{tabular}
	}
	\end{adjustbox}
\end{table}

\begin{table}[H]
	\centering
	\caption{A patch code example of P11, Bitcoin \#12561}
	\label{tab:p11exp}
    \vspace{-2ex}
	% \resizebox{\linewidth}{!}{%
	\begin{adjustbox}{center} %angle=90
	\scalebox{0.7}{
		\begin{tabular}{c|l|}
			% \multicolumn{2}{l}{Bitcoin commit 5d322821:} \\
			\cline{2-2}
			  & \texttt{bool CChainState::ConnectBlock(const CBlock\& block, CValidationState\& ...)}                                   \\
			  & \texttt{\{}                                                                     \\
			  & \texttt{\hspace{5mm}...}                                                        \\
			- & \texttt{\hspace{5mm}if (!CheckBlock(block, state, chainparams.GetConsensus(), ...)} \\
			+ & \texttt{\hspace{5mm}if (!CheckBlock(block, state, chainparams.GetConsensus(), ...)) \{} \\
			+ & \texttt{\hspace{10mm}if (state.CorruptionPossible()) \{} \\
			+ & \texttt{\hspace{15mm}// We don't write down blocks to disk if they may have been} \\
			+ & \texttt{\hspace{15mm}// corrupted...} \\
			+ & \texttt{\hspace{15mm}return AbortNode(state, ...);}          \\
			+ & \texttt{\hspace{10mm}\}}          \\
			  & \texttt{\hspace{5mm}...}  \\
			  & \texttt{\}} \\
		    \cline{2-2}                                                                   
		\end{tabular}%
	}
	\end{adjustbox}
\end{table}

\begin{table}[H]
	\centering
	\caption{A patch code example of P19, Stellar \#2233}
	\label{tab:p19exp}
    \vspace{-2ex}
	% \resizebox{\linewidth}{!}{%
	\begin{adjustbox}{center} %angle=90
	\scalebox{0.7}{
		\begin{tabular}{c|l|}
			% \multicolumn{2}{l}{Bitcoin commit 5d322821:} \\
			\cline{2-2}
			  & \texttt{Config::validateConfig(bool mixed) \{}                                   \\
			  & \texttt{\hspace{5mm}...}                                                        \\
			+ & \texttt{\hspace{5mm}if (!isQuorumSetSane(QUORUM\_SET, !UNSAFE\_QUORUM))} \\
			+ & \texttt{\hspace{5mm}\{} \\
			+ & \texttt{\hspace{10mm}LOG(FATAL) << fmt::format("Invalid QUORUM\_SET: check nesting, "\hspace{9mm}} \\
			+ & \texttt{\hspace{15mm}"duplicate entries and thresholds (must be "} \\
			+ & \texttt{\hspace{15mm}"between {} and 100)",} \\
			+ & \texttt{\hspace{15mm}UNSAFE\_QUORUM ? 1 : 51);} \\
			+ & \texttt{\hspace{10mm}throw std::invalid\_argument("Invalid QUORUM\_SET");} \\
			+ & \texttt{\hspace{5mm}\}}          \\
			  & \texttt{\hspace{5mm}...}  \\
			  & \texttt{\}} \\
		    \cline{2-2}                                                                   
		\end{tabular}%
	}
	\end{adjustbox}
\end{table}

\begin{table}[H]
	\centering
	\caption{A patch code example of P20, Ethereum \#19401}
	\label{tab:p20exp}
    \vspace{-2ex}
	% \resizebox{\linewidth}{!}{
	\begin{adjustbox}{center} %angle=90
	\scalebox{0.7}{
		\begin{tabular}{c|l|}
			% \multicolumn{2}{l}{Ethereum commit b155b9d8:} \\
			\cline{2-2}
			  & \texttt{func (s *PublicBlockChainAPI) EstimateGas(ctx context.Context, ...) ... \{}                                                     \\
			+ & \texttt{\hspace{5mm}if gasCap := s.b.RPCGasCap(); gasCap != nil \{}         \\
			+ & \texttt{\hspace{10mm}if *args.Gas.Cmp(gasCap) > 0 \{} \\
			+ & \texttt{\hspace{15mm}log.Warn("Applying cap on gas, caller requested amount above ...)} \\
			+ & \texttt{\hspace{15mm}newGas := hexutil.Uint64(gasCap.Uint64())} \\
			+ & \texttt{\hspace{15mm}*args.Gas = newGas} \\
			+ & \texttt{\hspace{10mm}\}} \\
			+ & \texttt{\hspace{5mm}\}}    \\
			  & \texttt{\hspace{5mm}return DoEstimateGas(ctx, s.b, args, rpc.PendingBlockNumber)}   \\
			  & \texttt{\}} \\
			\cline{2-2}                                                       
		\end{tabular}
	}
	\end{adjustbox}
\end{table}

\begin{table}[H]
	\centering
	\caption{A patch code example of P21, Monero \#706}
	\label{tab:p21exp}
    \vspace{-2ex}
	% \resizebox{\linewidth}{!}{
	\begin{adjustbox}{center} %angle=90
	\scalebox{0.7}{
		\begin{tabular}{c|l|}
			% \multicolumn{2}{l}{Ethereum commit b155b9d8:} \\
			\cline{2-2}
			  & \texttt{void Blockchain::check\_against\_checkpoints(const checkpoints\& points, ...) \{}                                                     \\
			  & \texttt{\hspace{5mm}const auto\& pts = points.get\_points();}         \\
			  & \texttt{\hspace{5mm}}         \\
			+ & \texttt{\hspace{5mm}CRITICAL\_REGION\_LOCAL(m\_blockchain\_lock);}                        \\
			  & \texttt{\hspace{5mm}m\_db->batch\_start();} \\
			  & \texttt{\hspace{5mm}for (const auto\& pt : pts) \{} \\
			  & \texttt{\hspace{5mm}...} \\
			  & \texttt{\}} \\
			\cline{2-2}                                                       
		\end{tabular}
	}
	\end{adjustbox}
\end{table}
